# Supplementary material for: Comparing the pre-SNe feedback and environmental pressures for 6000 HII regions across 19 nearby spiral galaxies
Source: arXiv:2110.05492 source file (2021-10-25)
Supplement: Supplementary file 1 [file appendix_old.tex]

\appendix

% \section{Unresolved structure}\label{sec:hstcomp}

% Throughout this work, we have made use of an \HII\ region catalogue that has been created by using the HIIphot algorithm \citep{Thilker2000} on our integral field \Ha\ maps from MUSE. The MUSE cubes have an angular resolution between 0.5\arcsec\ (using adaptive optics) to 1\arcsec, which, at the distances of our sample, corresponds to physical scales of several tens of pc (see Table\,\ref{tab:galprops}). It is, however, highly likely that observations at these scales do not fully resolve the internal structure of many of the \HII\ regions. We have addressed this for the smallest \HII\ regions within our sample by labelling them as ``unresolved'' (i.e.\ $r_\mathrm{eff}/r_\mathrm{eff,min}>2$; see section\,\ref{sec:selection_bias}), and determining their sizes via an alternative method (see section\,\ref{sec:lowerlimits}). However, even those that have a morphology that extends significantly beyond the MUSE resolution and are, hence, classified as ``resolved'' in our analysis, may be still partially unresolved and/or contain substructure. 

% To investigate the presence of unresolved substructure, we compare the MUSE \Ha\ emission map across NGC3351 to a (continuum subtracted, yet not extinction corrected) \Ha\ map obtained with the Hubble Space Telescope (HST). Figure\,\ref{fig:hstcomp} shows the comparison of these two datasets for several \HII\ regions from our sample that were classified as being resolved. These HST observations have around an order of magnitude higher angular resolution (0.06\arcsec) compared to the MUSE observations taken using AO (0.6\arcsec), which at the distance of NGC3351 corresponds to a spatial resolution of around $\sim$\,3\,pc (see Table\,\ref{tab:galprops}). However, the HST observations are much shallower than the MUSE observations, and, therefore, only recover the brightest features across the galaxy. Nonetheless, Figure\,\ref{fig:hstcomp} shows that much of the bright emission within the HST maps has a complex morphology that is not seen within the MUSE observations. We see that the approximately circular \HII\ regions seen within the MUSE maps, appear to be, in fact, open ring-like structures within the HST maps. The ring part of these structures could correspond to e.g.\ the limb brightened shells of the \HII\ regions, and their openings could be blistered regions where the ionised gas could be leaking into the surrounding medium (a potential cause for the significant low-level emission of diffuse ionised gas observed in the MUSE observations). Moreover, in Figure\,\ref{fig:hstcomp} we compare to the IBV broadband emission from the HST, where blue (i.e.\ from the 814\,nm band) corresponds to young stellar clusters. Interestingly, we see that the structure of the \HII\ regions seen in the \Ha\ emission from HST appears to surround the bright clusters.

% Qualitatively, it is clear from Figure\,\ref{fig:hstcomp} that the sizes of the \HII\ regions within NGC3351 seen with the HST observations are systematically smaller than those observed with MUSE. However, a quantitative comparison between the sizes measured with MUSE and those measurable with HST is non-trivial primarily due to two reasons: the different sensitivity limits of these two sets of observations, and the complex structures that are resolved within the HST observations. The first complicates a systematic comparison of the same emission within both datasets, as, for example, the MUSE observations recover a significant fraction of the diffuse ionised gas surrounding the \HII\ regions that is not detected by HST observations. Although the inclusion of extended diffuse emission has been limited by our source identification routine, it is likely that some fraction remains and artificially increases the size of the \HII\ regions measured with MUSE. Secondly, the complex structures seen within the HST observations make an accurate and reliable determination of their sizes difficult. In addition, as they are not simple Gaussian-like structures, they do not simply correspond to the sizes measured by MUSE deconvolved by the MUSE point spread function.

% In light of the above, we defer an in-depth comparison of the \HII\ regions observed within the MUSE and HST observations to future work, and here compare the MUSE sizes provided from our source identification to manually determined size estimates in the HST observations. For this analysis, we choose a subsample of 15 \HII\ regions from the catalogue that have been classified as resolved, isolated, not in the central part of the galaxy, and appear bright within the shallow HST images. For each region, in the HST image, we then identified the radius of the source at a contour level of 0.01\,s$^{-1}$ counts ($r_\mathrm{circ,HST}^\mathrm{in}$ and $r_\mathrm{circ,HST}^\mathrm{out}$, respectively). In Figure\,\ref{fig:hstcompscatter}, we plot the MUSE $r_\mathrm{eff}$ as a function of the $r_\mathrm{circ,HST}$ estimates. We see that ratios of $r_\mathrm{circ,HST}/r_\mathrm{eff,MUSE}$ range between 0.5 to 1, with a mean value of around 0.75. We, therefore, infer that the sizes of the resolved sample could be typically overestimated by around 25\,per cent. With that said, however, we have only conducted this analysis on a single galaxy for which continuum subtracted \Ha\ observations from the HST were readily available, and this result is expected to change significantly between galaxies; e.g.\ depending on the distance.  

% \input{./figs/fig_hstcomp.tex}

% \section{Varying upper limits}\label{sec:sizelimits}

% Throughout this work, we make use of lower limit estimates for the sizes of the \HII\ region sample. These are determined using the expression for a Strömgren sphere \citep{stromgren_1939}, and solving for $r_\mathrm{eff}$ where a measurement of $n_\mathrm{e}$ has been possible. The lower limits are a result of not knowing the filling factor of the ionized gas (i.e.\ $r_\mathrm{eff}\propto1/f$). In this section, we examine how these limits affect the various pressure components. 

% We investigate the effect of assuming that the sizes of the \HII\ regions are significantly larger than their lower limit. In Figure\,\ref{fig:limits}, we show the effect of using the measured size of the unresolved \HII\ regions, instead of their lower limits. As they are unresolved, their measured sizes correspond to a point source and, hence, this represents an upper limit on the size. We see that increasing the sizes of the \HII\ regions does not affect the measured \ptherm, hence in the pressure--size parameter space, these lower limit points only move to the right (see Figure\,\ref{fig:limits}). Yet, for \pdir, increasing the sizes of the \HII\ regions \pdir\ points also has the effect of decreasing the pressure because of its $r_\mathrm{eff}^{-2}$ dependence. In Figure\,\ref{fig:limits}, these points then move both to the right and down, and, therefore, move even further below the \pdir\ limits. This then strengthens the conclusion within the paper that these \HII\ regions are typically dominated by thermal pressure, as opposed to the direct radiation pressure.  

% \section{Luminosity conversion}\label{sec:lumconv}

% The calculation of the direct radiation pressure requires an estimate for the bolometric luminosity, which we assume is given as $L_\mathrm{bol} = \left<h\nu\right> Q(\mathrm{H}^o)$, were $\left<h\nu\right>$\,$\sim$\,15\,eV is the mean photon energy, and $Q(\mathrm{H}^o)$ is the ionising
% photon rate. The conversion use is then approximately equal to $L_\mathrm{bol} \approx 18 L_\mathrm{H_\upalpha}$. This, however, differs from the conversion presented by \citet{kennicutt_2012}, which accounts for a stellar population that fully samples the initial mass function (IMF), and the stellar age distribution. This conversion is given as $L_\mathrm{bol,IMF} \approx 138 L_\mathrm{H_\upalpha}$, and is a factor of $\sim$\,8 higher than the conversion purely from the massive stars used in this work. Given that the \HII\ regions in this work are assumed to be relatively young, their stellar populations may sample only a part of the IMF. In reality, we expect the correct conversion should it somewhere between $L_\mathrm{bol}$ and $L_\mathrm{bol,IMF}$, and should vary between the \HII\ regions. Figure\,\ref{fig:limits} shows the effect of assuming both $L_\mathrm{bol}$ and $L_\mathrm{bol,IMF}$ for the determination of the direct radiation pressure. We see that the upper limits of \pdir\ are similar to the \ptherm\ (note the aforementioned behaviour of these limits), yet where we have measurements \pdir<\ptherm. Again, this then confirms the conclusion these \HII\ regions are typically dominated by thermal pressure, as opposed to direct radiation pressure.  

% \input{./figs/fig_presscaterr.tex}
% \input{./figs/fig_presscatindv.tex}
% \input{./figs/fig_prophist.tex}

% \section{Tables}

% Within this work, we have determined several properties for a large sample of \HII\ regions identified across 19 nearby spiral galaxies. In Tables\,\ref{tab:obsprops} and \ref{tab:phyprops} we summarise the measured and derived quantities for $\sim$\,5000 \HII\ regions that meet the selection criteria outlined in section\,\ref{sec:selection_bias}. These tables are available in a full machine-readable format in the online supplementary material. 

% \input{./tabs/tab_obsprops.tex}
% \input{./tabs/tab_physprops.tex}
